# Supplementary material for: The Impact of Sub-Resolution Porosity on Numerical Simulations of Multiphase Flow
Source: arXiv:2109.13903 source file (2021-09-28)
Supplement: Supplementary file 1 [file SM.tex]

 %% 
%% Copyright 2007, 2008, 2009 Elsevier Ltd
%% 
%% This file is part of the 'Elsarticle Bundle'.
%% ---------------------------------------------
%% 
%% It may be distributed under the conditions of the LaTeX Project Public
%% License, either version 1.2 of this license or (at your option) any
%% later version.  The latest version of this license is in
%%    http://www.latex-project.org/lppl.txt
%% and version 1.2 or later is part of all distributions of LaTeX
%% version 1999/12/01 or later.
%% 
%% The list of all files belonging to the 'Elsarticle Bundle' is
%% given in the file `manifest.txt'.
%% 
%% Template article for Elsevier's document class `elsarticle'
%% with harvard style bibliographic references
%% SP 2008/03/01

%\documentclass[preprint,review,12pt,authoryear]{elsarticle}

%% Use the option review to obtain double line spacing
%% \documentclass[authoryear,preprint,review,12pt]{elsarticle}

%% Use the options 1p,twocolumn; 3p; 3p,twocolumn; 5p; or 5p,twocolumn
%% for a journal layout:
\documentclass[final,1p,times,authoryear]{elsarticle}
%\documentclass[final,1p,times,twocolumn,authoryear]{elsarticle}
%\documentclass[final,5p,twocolumn,6pt,authoryear]{elsarticle}
%\documentclass[final,3p,times,authoryear]{elsarticle}
%% \documentclass[final,3p,times,twocolumn,authoryear]{elsarticle}
%% \documentclass[final,5p,times,authoryear]{elsarticle}
%% \documentclass[final,5p,times,twocolumn,authoryear]{elsarticle}

%% For including figures, graphicx.sty has been loaded in
%% elsarticle.cls. If you prefer to use the old commands
%% please give \usepackage{epsfig}

\pdfoutput=1


%% The amssymb package provides various useful mathematical symbols
\usepackage{fullpage}
\usepackage{amssymb}
\usepackage{amsmath}
\usepackage{lipsum}
\usepackage{nomencl}
\usepackage{pstricks}
\usepackage{tablefootnote}
\usepackage[colorlinks=true,linkcolor=blue,citecolor=blue,allcolors=blue]{hyperref}
\usepackage{siunitx}
\usepackage{cellspace}
\usepackage{amsmath, array, makecell}
\usepackage{multibib}
\usepackage[]{graphicx}
\usepackage{nomencl}
\makenomenclature
\usepackage{verbatim}

\renewcommand{\nomname}{List of Symbols}

\usepackage{lipsum}

\usepackage{units}
%\usepackage[T1]{fontenc}
\usepackage[utf8]{inputenc}
\usepackage{multirow}
\usepackage{dsfont}
%\usepackage{amssymb}
%% The amsthm package provides extended theorem environments
%% \usepackage{amsthm}

%% The lineno packages adds line numbers. Start line numbering with
%% \begin{linenumbers}, end it with \end{linenumbers}. Or switch it on
%% for the whole article with \linenumbers.
\usepackage{lineno}
%\linenumbers

\usepackage{setspace}
\onehalfspacing
%\renewcommand{\nomgroup}[1]{%
%\ifthenelse{\equal{#1}{A}}{\item[\textbf{Variables}]}{%
%\ifthenelse{\equal{#1}{S}}{\item[\textbf{Subscripts}]}{
%\ifthenelse{\equal{#1}{Z}}{\item[\textbf{Abbreviations}]}}}}
\makenomenclature
%% The amsthm package provides extended theorem environments
%% \usepackage{amsthm}

%% The lineno packages adds line numbers. Start line numbering with
%% \begin{linenumbers}, end it with \end{linenumbers}. Or switch it on
%% for the whole article with \linenumbers.
%% \usepackage{lineno}

\journal{Advances in Water Resources}

\begin{document}

\begin{frontmatter}

%% Title, authors and addresses
\title{Supplementary Materials for: ``The Impact of Sub-Resolution Porosity on Numerical Simulations of Multiphase Flow"}

\author[PRINCETONCIVIL]{Francisco J. Carrillo}
\author[CNRS]{Cyprien Soulaine}
\author[PRINCETONCIVIL,HMEI]{Ian C. Bourg}

\address[PRINCETONCIVIL]{Department of Civil and Environmental Engineering, Princeton University, Princeton, NJ, USA}
\address[PEI]{High Meadows Environmental Institute, Princeton University, Princeton, NJ, USA}
\address[CNRS]{Earth Sciences Institute of Orl\'eans, Universit\'e d'Orl\'eans, CNRS, BRGM, Orl\'eans, France}

\begin{abstract}
This Supplementary Material consists of the following:
\begin{enumerate}
 
\item A \hyperref[additionalrelperm]{Figure} containing additional relative permeability curves.

\item A \hyperref[times]{Figure} that depicts the impact of SRP on oil breakthrough times. 

\item A \hyperref[residualwater]{Figure} that depicts the impact of SRP on residual water saturations.

\end{enumerate}

\end{abstract}

\end{frontmatter}

\newpage

\section{Additional Relative Permeability Curves}\label{additionalrelperm}

\begin{figure}[htb]
\begin{center}
\includegraphics[width=0.6\textwidth]{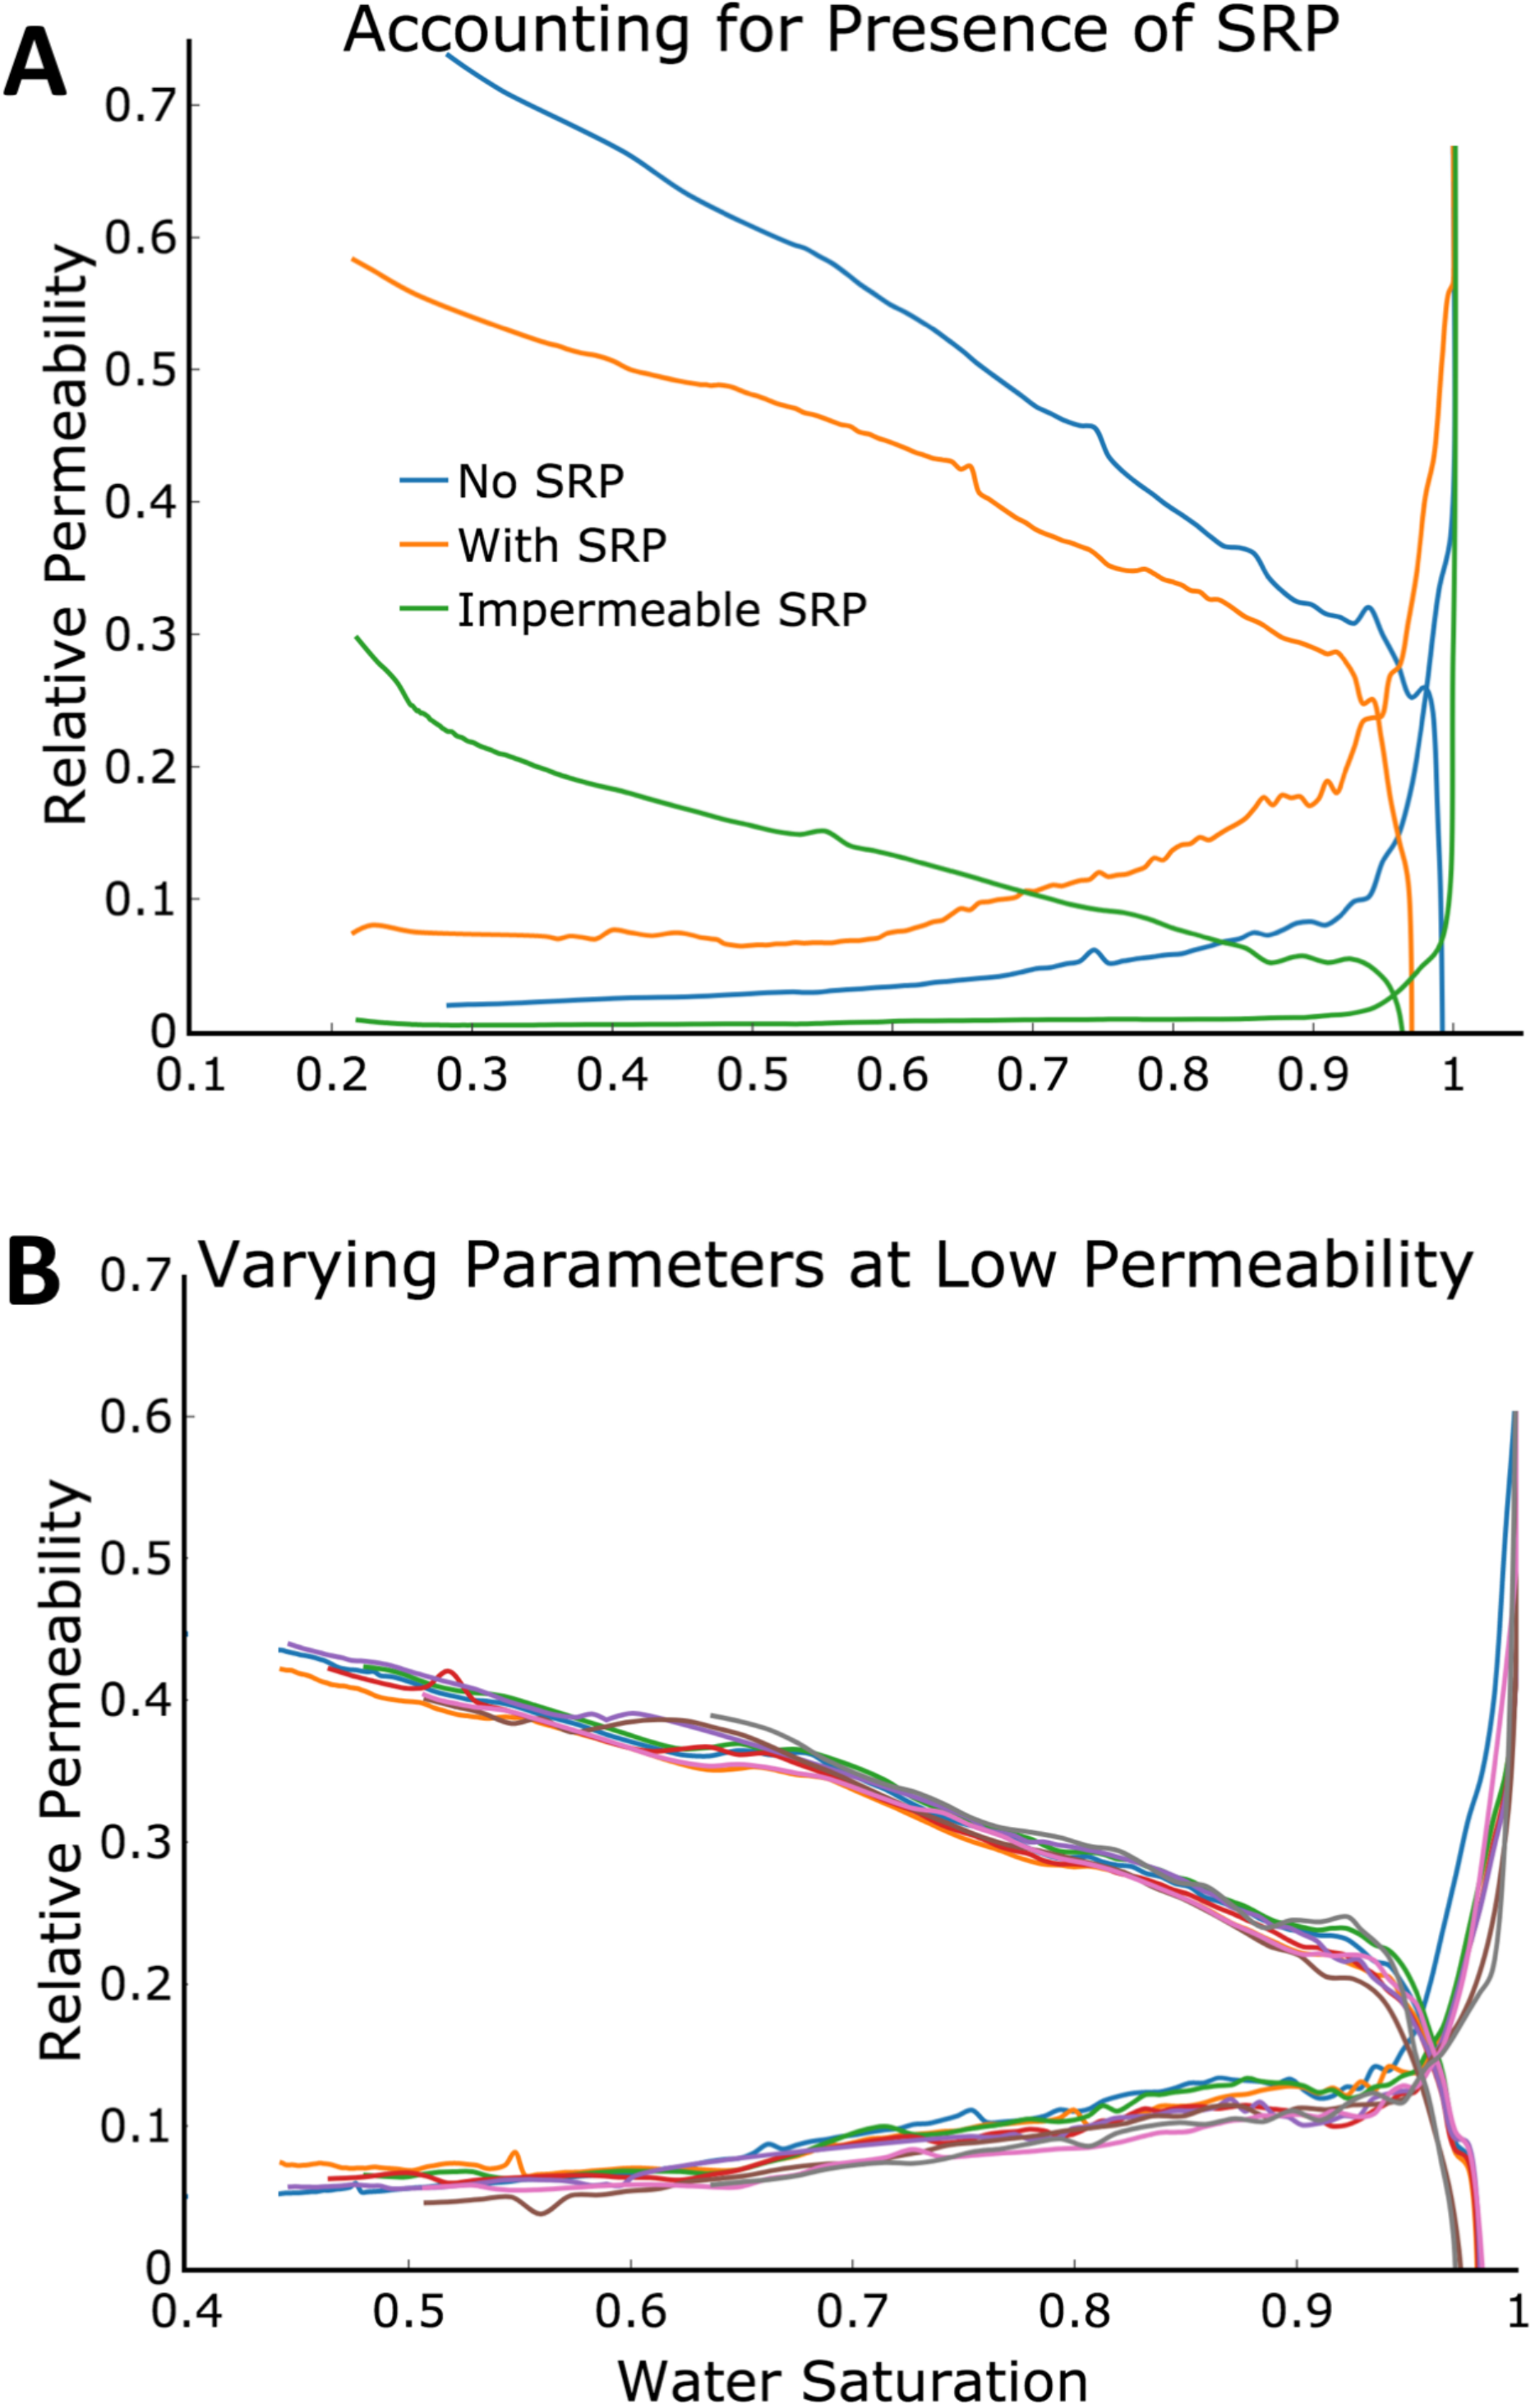}
\caption{A) The effects of removing the SRP ($\phi =1$) and solidifying the SRP ($\phi = 0$). B) The effects of changing the wettability properties of an SRP with an absolute permeability of $k_0 = 1\times10^{-17} \ m^2$.   Unless specified, all parameterized values not indicated in the legend are held constant and equal to the values described in Tables 1 and 2 in the main text. Each color pair represents the oil (top) and water (bottom) relative permeability curves for a given simulated case.}
\end{center} 
\end{figure}

\newpage

\section{SRP Impact on Oil Breakthrough Times}\label{times}

\begin{figure}[h!]
\includegraphics[width=0.9\textwidth]{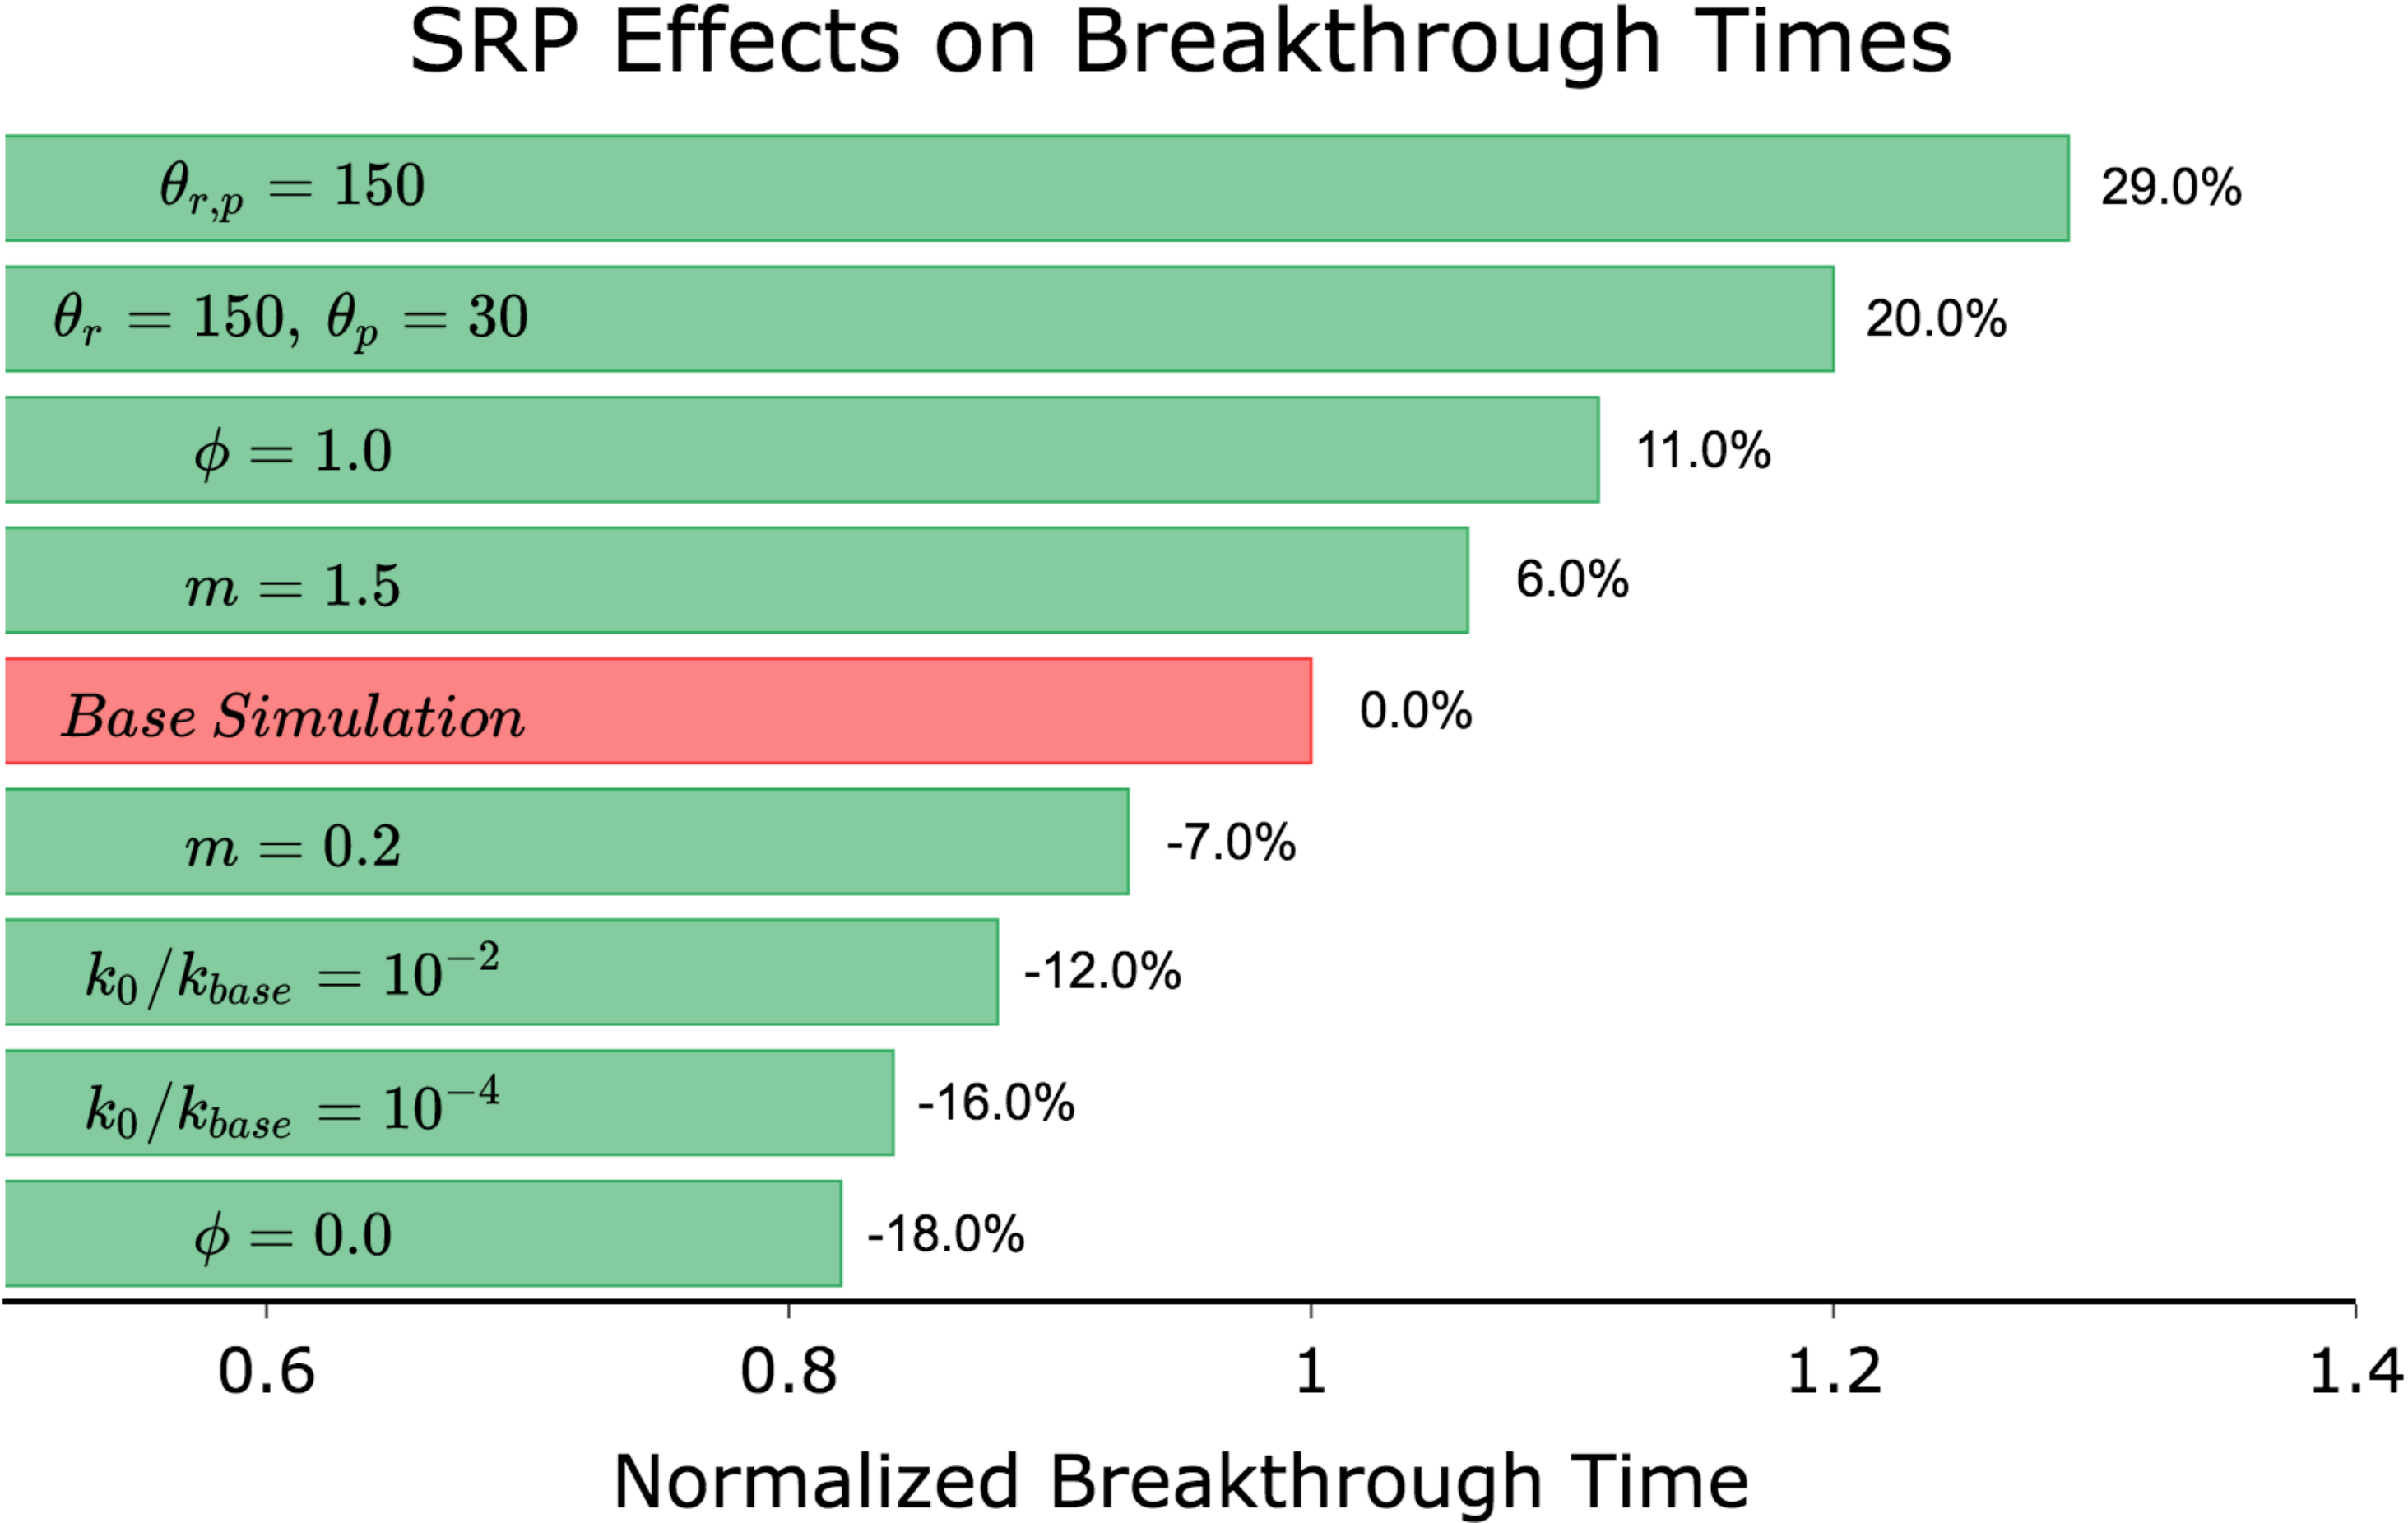}
\caption{\label{fig:breakthrough_time} Normalized oil breakthrough times for select cases. Each label shows the only varied parameter with respect to the base simulation. The percentages to the right of the bars show the percent change in breakthrough time with respect to the aforementioned base simulation specified in Section 3.}
\end{figure}

\newpage

\section{SRP Impact Residual Water Saturations}\label{residualwater}

\begin{figure}[h!]
\begin{center}
\includegraphics[width=0.9\textwidth]{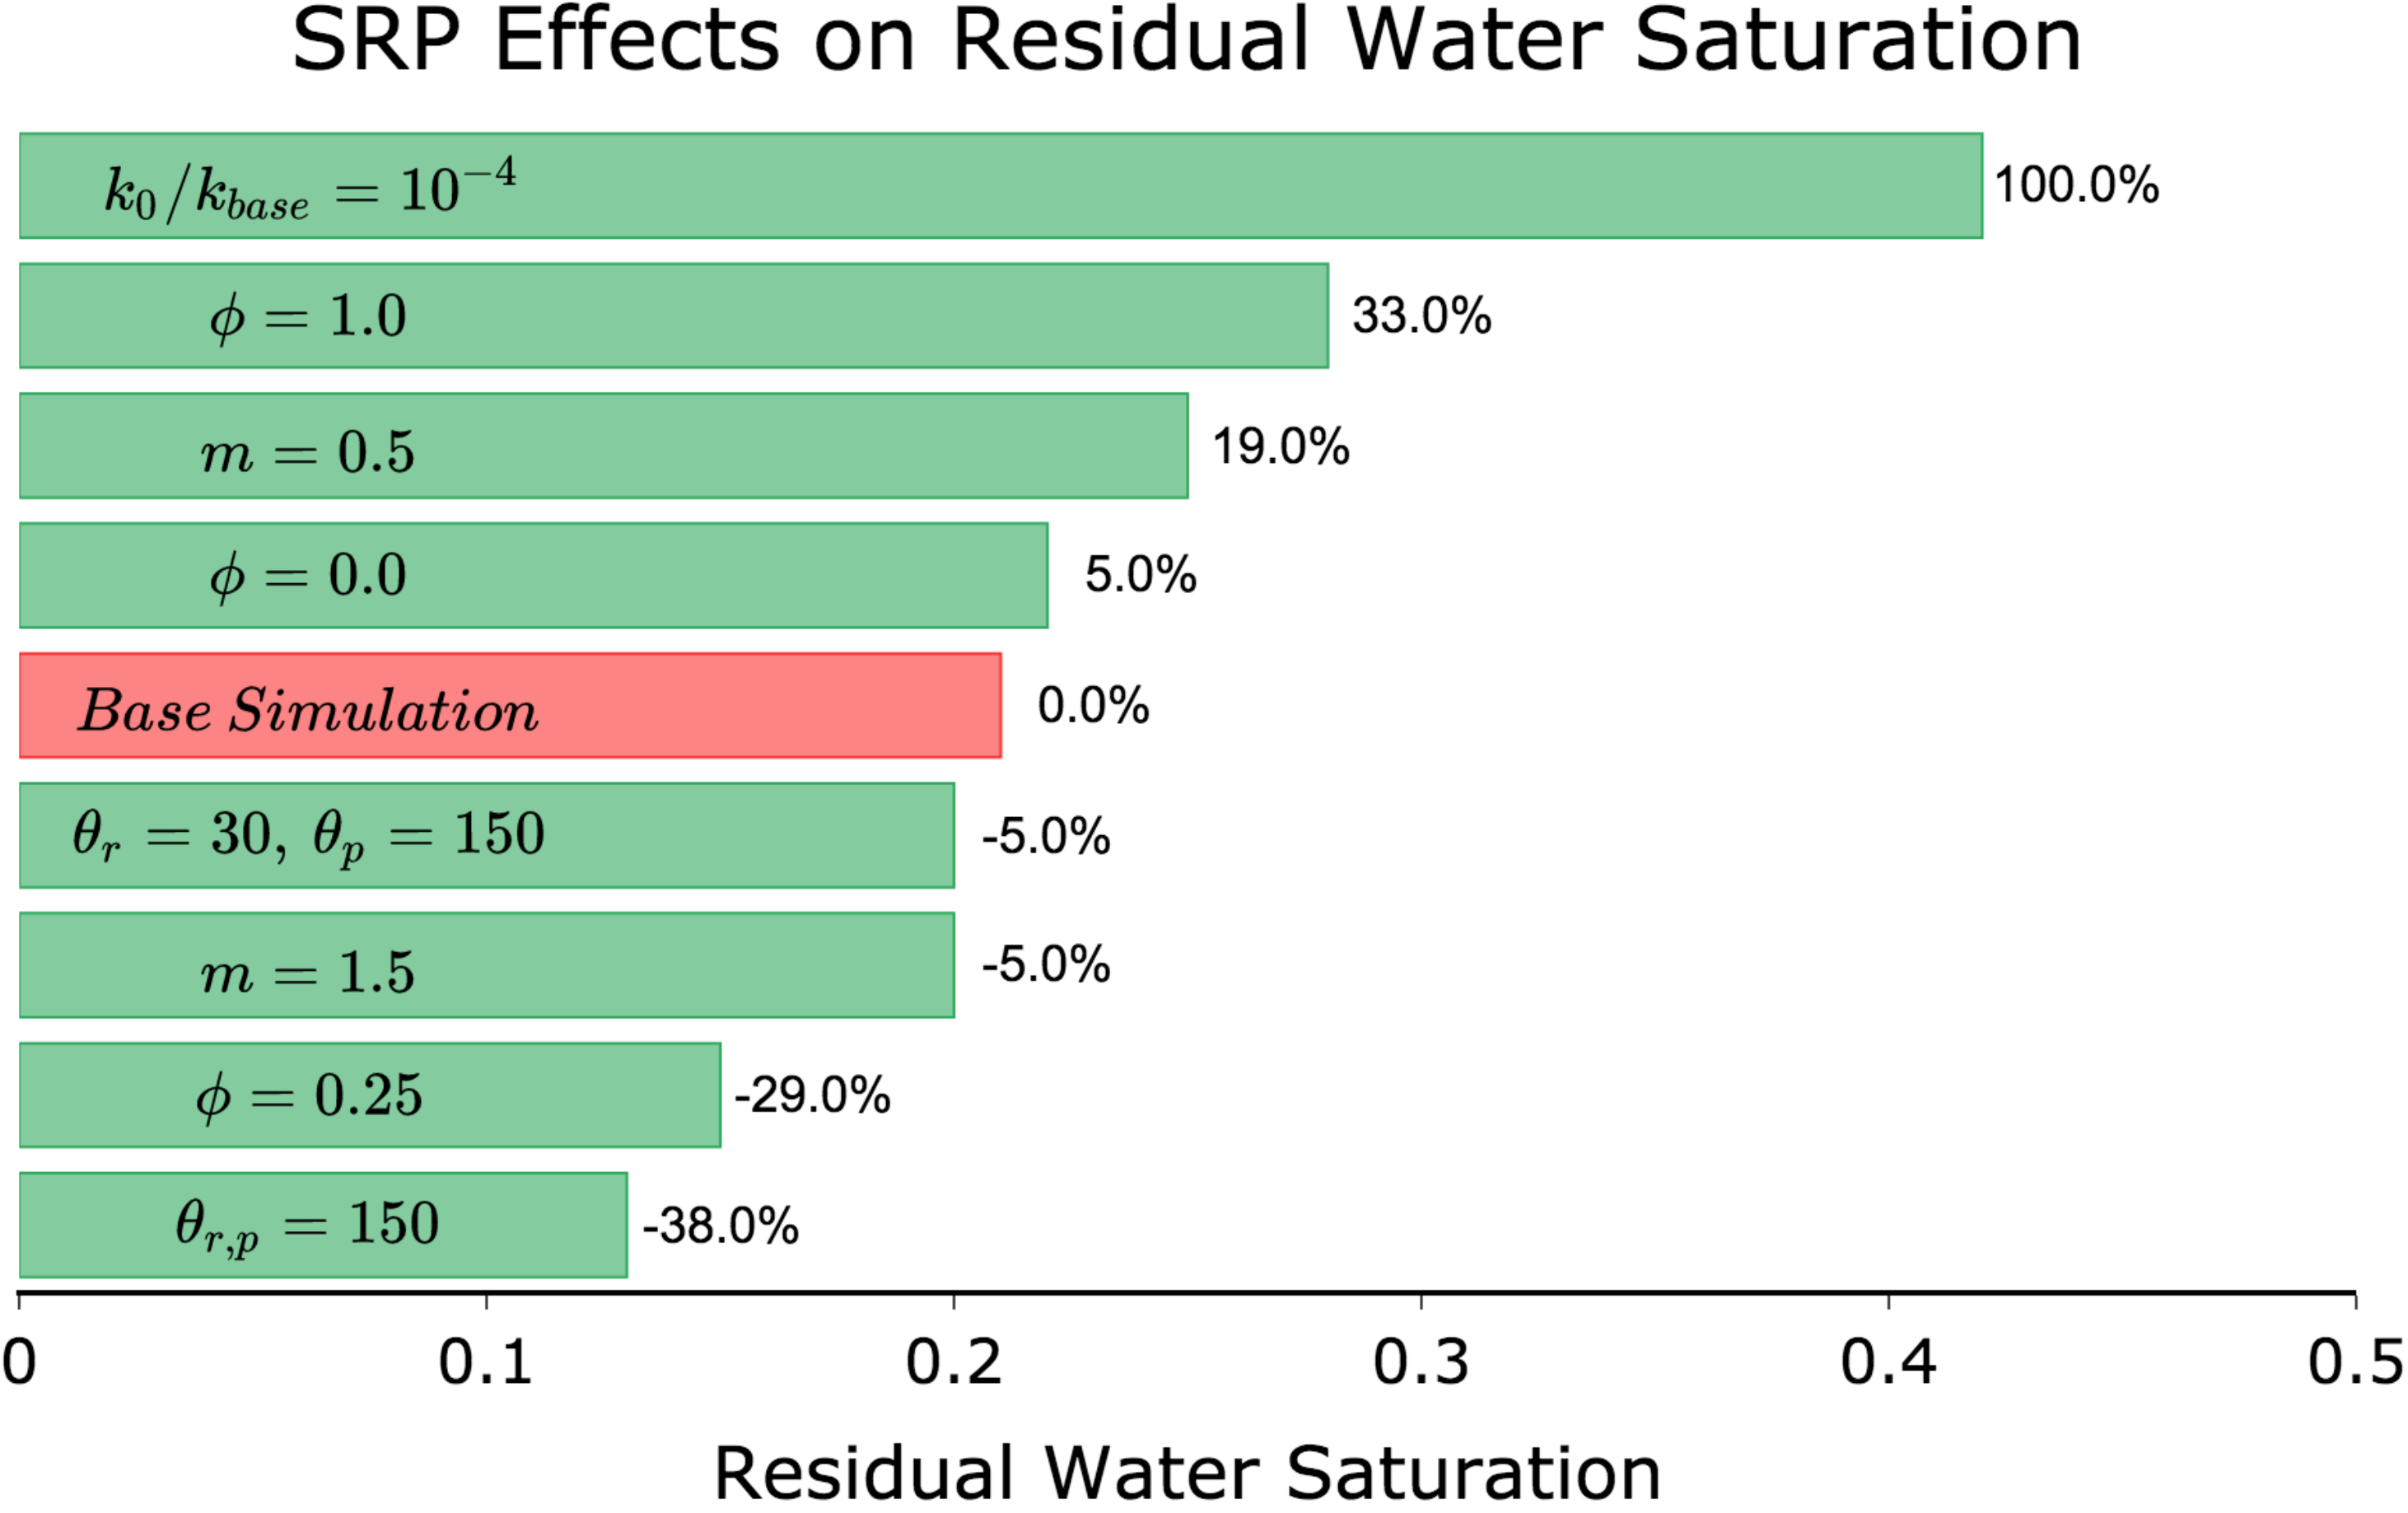}
\caption{\label{fig:residual_saturations} Residual water saturations for select cases. Each label shows the only varied parameter with respect to the base simulation. The percentages to the right of the bars show the percent change in residual saturations with respect to the base simulation specified in Section 3.}
\end{center}
\end{figure}

%\section*{References}
\bibliographystyle{elsarticle-harv}
\bibliography{ref,Sibib}

\end{document}
\endinput
